# Supplementary material for: Verifiable Learning for Robust Tree Ensembles
Source: arXiv:2305.03626 source file (2023-11-11)
Supplement: Supplementary file 1 [file additional_experiments.tex]

\section{Experiments with other norms}
\LC{Sezione provvisoria, conterrà tabelle o plot di nuovi risultati sperimentali}
